# Supplementary material for: Bias correction of satellite and reanalysis products for daily rainfall occurrence and intensity
Source: arXiv:2510.27456 source file (2025-12-23)
Supplement: Supplementary file 1 [file Supplementary_Material.pdf]

# Supplementary Material for Bias correction of satellite and reanalysis products for daily rainfall occurrence and intensity

John Bagiliko <sup>a, b</sup>, David Stern <sup>c</sup>, Denis Ndanguza <sup>a</sup>, Francis Feehi Torgbor <sup>d</sup>,  
Danny Parsons <sup>a, b, c</sup>, Samuel Owusu Ansah <sup>e</sup>

<sup>a</sup> Department of Mathematics, School of Science, College of Science and Technology,  
University of Rwanda, P.O. Box 3900, Kigali, Rwanda

<sup>b</sup> African Institute for Mathematical Sciences, Research and Innovation Center, Rue  
KG590 ST, Kigali, Rwanda

<sup>c</sup> IDEMS International, RG2 7AX, Reading, United Kingdom

<sup>d</sup> Ghana Innovations in Development, Education and the Mathematical Sciences, Okponglo,  
East Legon, Accra, Ghana

<sup>e</sup> Ghana Meteorological Agency, P.O. Box LG 87, Accra, Ghana

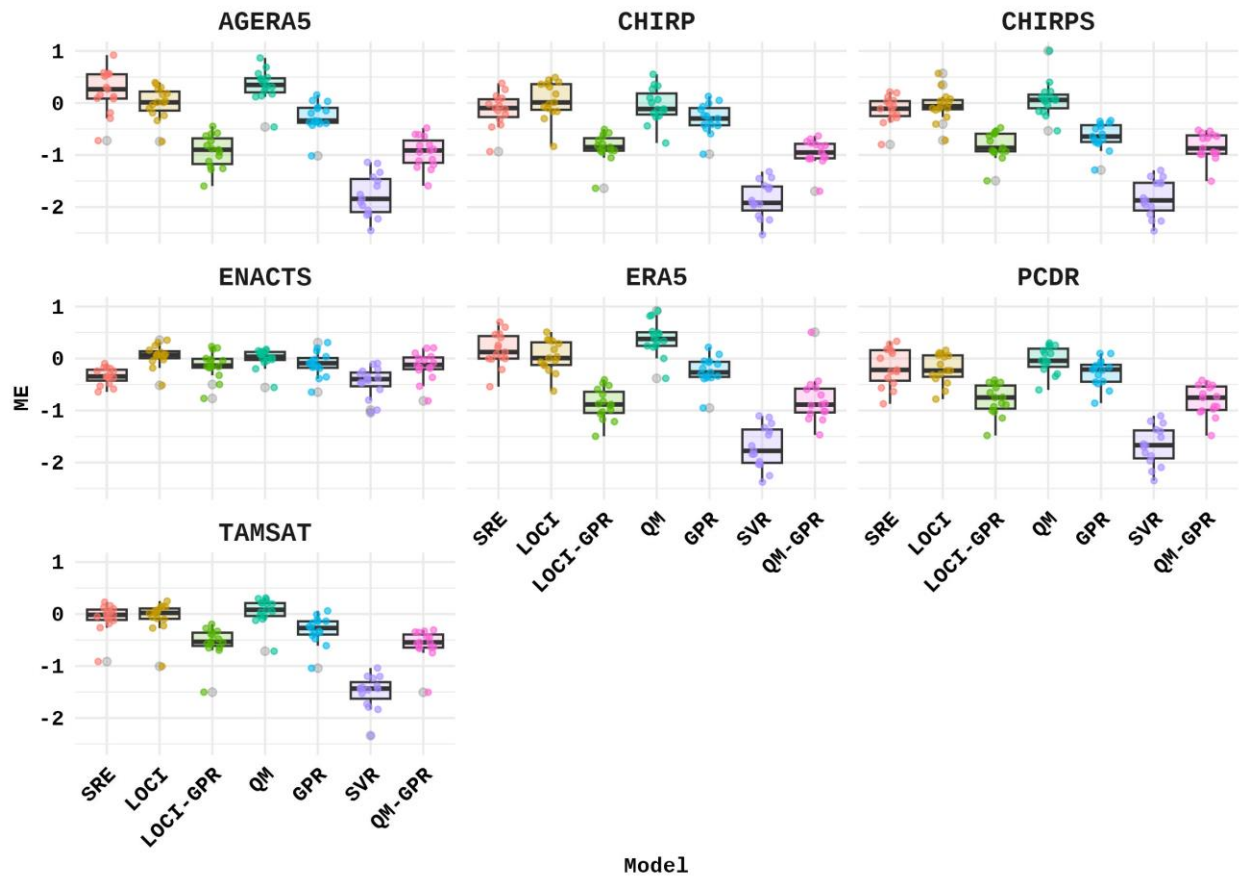

Figure S1: Box plots showing the MEs of the BC methods applied to the SREs in Zambia

Table S1: Overall performance metrics by SRE and BC method at the daily scale in Zambia

| Product | Model | ME | MAE | RMSE | Corr | NSE | RSD |
|---------|-------|----|-----|------|------|-----|-----|
|---------|-------|----|-----|------|------|-----|-----|

|        |          |        |       |        |       |        |       |
|--------|----------|--------|-------|--------|-------|--------|-------|
| CHIRPS | SRE      | -0.129 | 3.162 | 8.289  | 0.431 | 0.133  | 0.659 |
| CHIRPS | LOCI     | -0.049 | 3.333 | 8.937  | 0.397 | -0.007 | 0.803 |
| CHIRPS | LOCI-GPR | -0.818 | 2.917 | 8.096  | 0.427 | 0.173  | 0.454 |
| CHIRPS | QM       | 0.075  | 3.606 | 10.559 | 0.351 | -0.406 | 1.079 |
| CHIRPS | GPR      | -0.644 | 2.95  | 8.036  | 0.438 | 0.185  | 0.477 |
| CHIRPS | SVR      | -1.853 | 2.701 | 8.493  | 0.373 | 0.09   | 0.296 |
| CHIRPS | QM-GPR   | -0.843 | 2.906 | 8.098  | 0.427 | 0.173  | 0.455 |
| CHIRP  | SRE      | -0.114 | 3.409 | 8.657  | 0.351 | 0.055  | 0.613 |
| CHIRP  | LOCI     | 0.067  | 3.749 | 9.857  | 0.295 | -0.226 | 0.855 |
| CHIRP  | LOCI-GPR | -0.852 | 3.116 | 8.374  | 0.357 | 0.116  | 0.412 |
| CHIRP  | QM       | -0.053 | 3.824 | 10.994 | 0.261 | -0.525 | 1.031 |
| CHIRP  | GPR      | -0.289 | 3.275 | 8.214  | 0.391 | 0.149  | 0.44  |
| CHIRP  | SVR      | -1.882 | 2.838 | 8.716  | 0.299 | 0.042  | 0.244 |
| CHIRP  | QM-GPR   | -0.967 | 3.068 | 8.395  | 0.355 | 0.111  | 0.409 |
| ERA5   | SRE      | 0.149  | 3.262 | 8.161  | 0.447 | 0.16   | 0.646 |
| ERA5   | LOCI     | 0.025  | 3.439 | 9.351  | 0.392 | -0.103 | 0.899 |
| ERA5   | LOCI-GPR | -0.894 | 2.922 | 8.101  | 0.428 | 0.172  | 0.451 |
| ERA5   | QM       | 0.376  | 3.834 | 11.921 | 0.344 | -0.792 | 1.297 |
| ERA5   | GPR      | -0.247 | 3.111 | 7.962  | 0.45  | 0.2    | 0.487 |
| ERA5   | SVR      | -1.731 | 2.748 | 8.479  | 0.364 | 0.093  | 0.326 |
| ERA5   | QM-GPR   | -0.814 | 2.967 | 8.334  | 0.39  | 0.124  | 0.53  |
| TAMSAT | SRE      | -0.062 | 2.98  | 7.877  | 0.493 | 0.218  | 0.652 |
| TAMSAT | LOCI     | -0.071 | 3.016 | 8.099  | 0.489 | 0.174  | 0.744 |
| TAMSAT | LOCI-GPR | -0.551 | 2.813 | 7.758  | 0.497 | 0.242  | 0.54  |
| TAMSAT | QM       | 0.049  | 3.309 | 9.816  | 0.413 | -0.214 | 1.032 |
| TAMSAT | GPR      | -0.313 | 2.892 | 7.746  | 0.497 | 0.244  | 0.54  |
| TAMSAT | SVR      | -1.511 | 2.627 | 8.135  | 0.448 | 0.166  | 0.372 |

|        |          |        |       |        |       |        |       |
|--------|----------|--------|-------|--------|-------|--------|-------|
| TAMSAT | QM-GPR   | -0.589 | 2.823 | 7.802  | 0.489 | 0.233  | 0.528 |
| ENACTS | SRE      | -0.333 | 2.066 | 6.07   | 0.74  | 0.542  | 0.672 |
| ENACTS | LOCI     | 0.058  | 2.108 | 6.084  | 0.739 | 0.54   | 0.812 |
| ENACTS | LOCI-GPR | -0.115 | 2.028 | 5.982  | 0.747 | 0.555  | 0.8   |
| ENACTS | QM       | -0.005 | 2.06  | 6.206  | 0.746 | 0.521  | 0.933 |
| ENACTS | GPR      | -0.094 | 2.031 | 5.953  | 0.75  | 0.56   | 0.794 |
| ENACTS | SVR      | -0.436 | 1.978 | 6.033  | 0.742 | 0.548  | 0.777 |
| ENACTS | QM-GPR   | -0.133 | 2.019 | 5.968  | 0.749 | 0.558  | 0.799 |
| PCDR   | SRE      | -0.174 | 3.112 | 8.088  | 0.44  | 0.176  | 0.572 |
| PCDR   | LOCI     | -0.213 | 3.271 | 8.834  | 0.391 | 0.017  | 0.759 |
| PCDR   | LOCI-GPR | -0.809 | 2.934 | 8.144  | 0.419 | 0.164  | 0.471 |
| PCDR   | QM       | -0.035 | 3.525 | 10.127 | 0.352 | -0.292 | 0.997 |
| PCDR   | GPR      | -0.28  | 3.073 | 7.934  | 0.456 | 0.207  | 0.468 |
| PCDR   | SVR      | -1.697 | 2.724 | 8.409  | 0.398 | 0.109  | 0.283 |
| PCDR   | QM-GPR   | -0.826 | 2.916 | 8.122  | 0.423 | 0.169  | 0.466 |
| AGERAS | SRE      | 0.209  | 3.415 | 8.476  | 0.403 | 0.094  | 0.663 |
| AGERAS | LOCI     | -0.011 | 3.565 | 9.645  | 0.342 | -0.173 | 0.881 |
| AGERAS | LOCI-GPR | -0.956 | 2.984 | 8.245  | 0.394 | 0.142  | 0.426 |
| AGERAS | QM       | 0.32   | 3.972 | 12.363 | 0.286 | -0.928 | 1.29  |
| AGERAS | GPR      | -0.28  | 3.187 | 8.165  | 0.407 | 0.159  | 0.482 |
| AGERAS | SVR      | -1.808 | 2.807 | 8.684  | 0.301 | 0.049  | 0.317 |
| AGERAS | QM-GPR   | -0.966 | 2.974 | 8.245  | 0.395 | 0.143  | 0.427 |

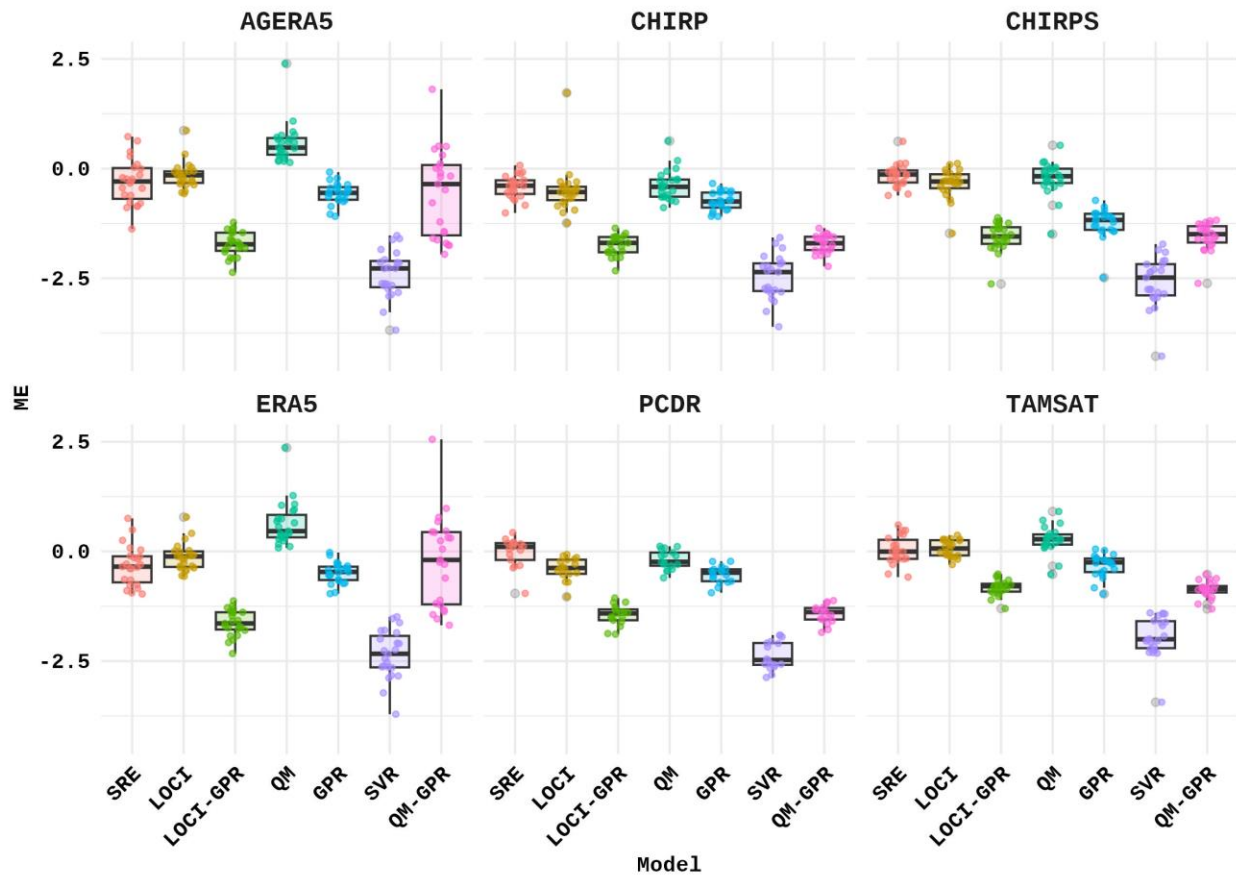

Figure S2: Box plots showing the MEs of the BC methods applied to the SREs in Ghana

Table S2: Performance metrics by SRE and BC methods at the daily scale in Ghana

| Product | Model    | ME     | MAE   | RMSE   | Corr  | NSE    | RSD   |
|---------|----------|--------|-------|--------|-------|--------|-------|
| CHIRPS  | SRE      | -0.156 | 4.046 | 10.165 | 0.328 | -0.031 | 0.699 |
| CHIRPS  | LOCI     | -0.343 | 4.093 | 10.982 | 0.283 | -0.203 | 0.814 |
| CHIRPS  | LOCI-GPR | -1.555 | 3.412 | 9.637  | 0.316 | 0.073  | 0.364 |
| CHIRPS  | QM       | -0.216 | 4.3   | 12.844 | 0.266 | -0.646 | 1.111 |
| CHIRPS  | GPR      | -1.234 | 3.53  | 9.519  | 0.335 | 0.096  | 0.371 |
| CHIRPS  | SVR      | -2.582 | 3.175 | 10.036 | 0.267 | -0.005 | 0.17  |
| CHIRPS  | QM-GPR   | -1.548 | 3.391 | 9.592  | 0.328 | 0.082  | 0.367 |
| CHIRP   | SRE      | -0.415 | 4.131 | 9.939  | 0.268 | 0.015  | 0.505 |
| CHIRP   | LOCI     | -0.486 | 4.347 | 30.846 | 0.061 | -8.457 | 2.97  |
| CHIRP   | LOCI-GPR | -1.743 | 3.519 | 9.842  | 0.264 | 0.037  | 0.312 |
| CHIRP   | QM       | -0.376 | 4.414 | 12.645 | 0.222 | -0.595 | 1.023 |
| CHIRP   | GPR      | -0.741 | 3.975 | 9.615  | 0.291 | 0.078  | 0.325 |

|        |          |        |       |        |       |        |       |
|--------|----------|--------|-------|--------|-------|--------|-------|
| CHIRP  | SVR      | -2.487 | 3.309 | 10.132 | 0.202 | -0.024 | 0.146 |
| CHIRP  | QM-GPR   | -1.717 | 3.499 | 9.797  | 0.272 | 0.043  | 0.317 |
| AGERA5 | SRE      | -0.313 | 4.216 | 10.345 | 0.233 | -0.067 | 0.58  |
| AGERA5 | LOCI     | -0.147 | 4.623 | 14.595 | 0.18  | -1.125 | 1.256 |
| AGERA5 | LOCI-GPR | -1.72  | 3.492 | 9.828  | 0.264 | 0.036  | 0.327 |
| AGERA5 | QM       | 0.583  | 5.305 | 20.878 | 0.15  | -3.349 | 1.986 |
| AGERA5 | GPR      | -0.566 | 4.051 | 9.644  | 0.282 | 0.072  | 0.346 |
| AGERA5 | SVR      | -2.409 | 3.352 | 10.178 | 0.158 | -0.033 | 0.181 |
| AGERA5 | QM-GPR   | -0.562 | 4.466 | 18.388 | 0.13  | -2.374 | 1.676 |
| ERA5   | SRE      | -0.331 | 4.082 | 9.891  | 0.312 | 0.037  | 0.554 |
| ERA5   | LOCI     | -0.123 | 4.461 | 13.671 | 0.262 | -0.839 | 1.215 |
| ERA5   | LOCI-GPR | -1.633 | 3.473 | 9.703  | 0.319 | 0.074  | 0.364 |
| ERA5   | QM       | 0.64   | 5.155 | 19.863 | 0.223 | -2.889 | 1.936 |
| ERA5   | GPR      | -0.488 | 4.028 | 9.55   | 0.329 | 0.103  | 0.389 |
| ERA5   | SVR      | -2.356 | 3.376 | 10.154 | 0.203 | -0.014 | 0.232 |
| ERA5   | QM-GPR   | -0.206 | 4.577 | 18.204 | 0.192 | -2.266 | 1.71  |
| PCDR   | SRE      | -0.023 | 4.11  | 9.433  | 0.339 | 0.054  | 0.587 |
| PCDR   | LOCI     | -0.394 | 4.105 | 10.561 | 0.287 | -0.186 | 0.803 |
| PCDR   | LOCI-GPR | -1.453 | 3.487 | 9.321  | 0.321 | 0.076  | 0.385 |
| PCDR   | QM       | -0.19  | 4.349 | 12.102 | 0.264 | -0.557 | 1.055 |
| PCDR   | GPR      | -0.531 | 3.924 | 9.128  | 0.345 | 0.114  | 0.387 |
| PCDR   | SVR      | -2.376 | 3.32  | 9.679  | 0.261 | 0.004  | 0.196 |
| PCDR   | QM-GPR   | -1.431 | 3.478 | 9.288  | 0.328 | 0.083  | 0.386 |
| TAMSAT | SRE      | 0.027  | 3.647 | 8.894  | 0.472 | 0.21   | 0.584 |

|        |          |        |       |       |       |        |       |
|--------|----------|--------|-------|-------|-------|--------|-------|
| TAMSAT | LOCI     | 0.067  | 3.688 | 9.633 | 0.452 | 0.073  | 0.813 |
| TAMSAT | LOCI-GPR | -0.822 | 3.291 | 8.938 | 0.46  | 0.202  | 0.514 |
| TAMSAT | QM       | 0.269  | 3.995 | 11.7  | 0.406 | -0.367 | 1.135 |
| TAMSAT | GPR      | -0.321 | 3.52  | 8.831 | 0.472 | 0.221  | 0.501 |
| TAMSAT | SVR      | -1.94  | 3.07  | 9.352 | 0.418 | 0.127  | 0.316 |
| TAMSAT | QM-GPR   | -0.868 | 3.27  | 8.928 | 0.462 | 0.204  | 0.507 |

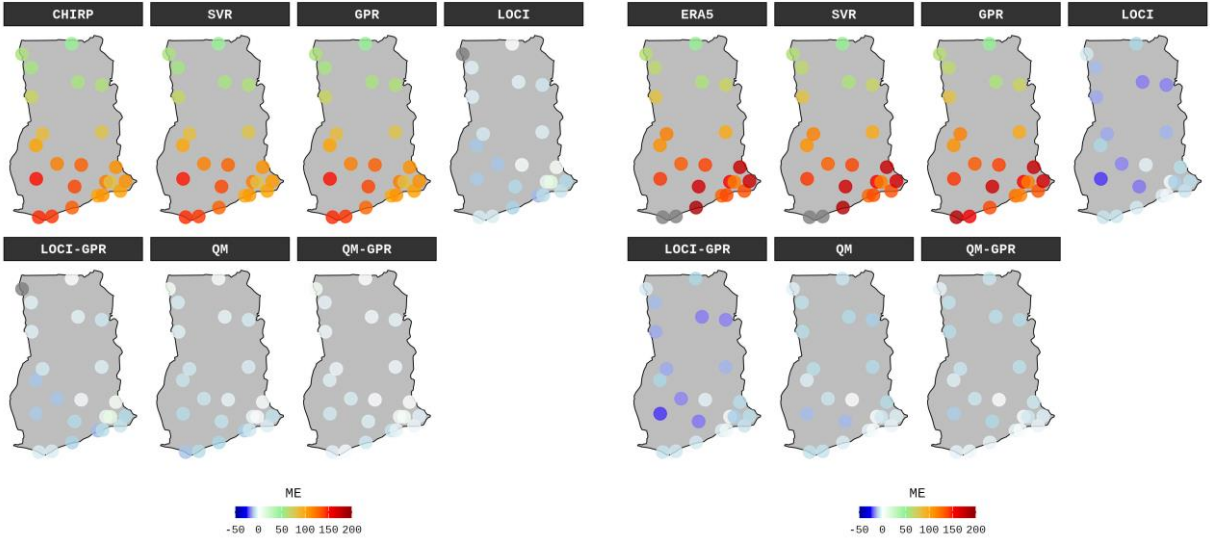

Figure S3: MEs on the annual number of rainy days across different stations in Ghana when the BC methods were applied on CHIRP

Figure S4: MEs on the annual number of rainy days across different stations in Ghana when the BC methods were applied on ERA5

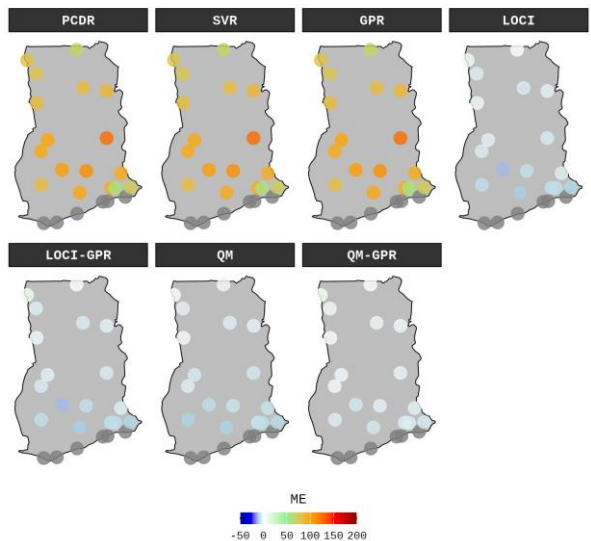

Figure S5: MEs on the annual number of rainy days across different stations in Ghana when the BC methods were applied on PCDR

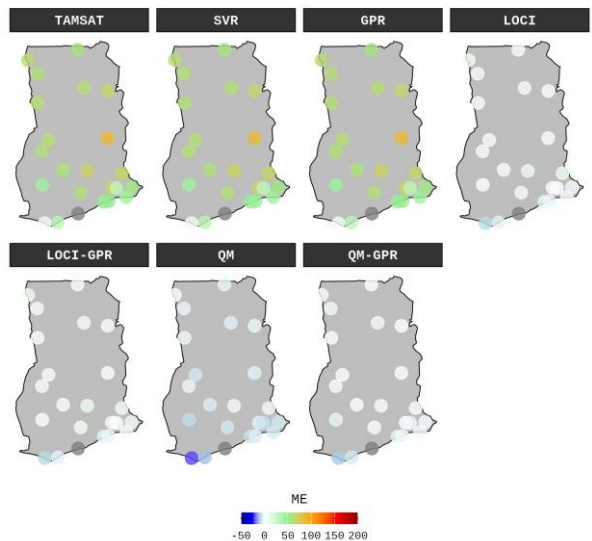

Figure S6: MEs on the annual number of rainy days across different stations in Ghana when the BC methods were applied on TAMSAT

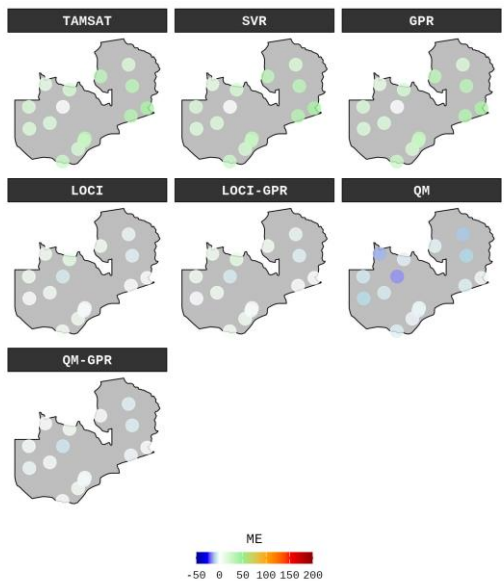

Figure S7: MEs on the annual number of rainy days across different stations in Zambia when the BC methods were applied on TAMSAT

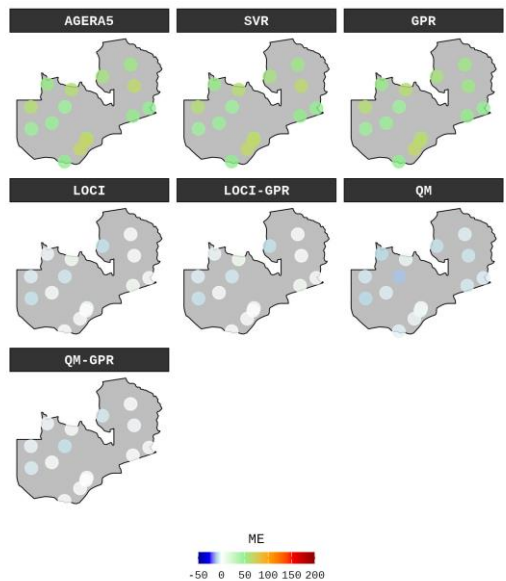

Figure S8: MEs on the annual number of rainy days across different stations in Zambia when the BC methods were applied on AGERA5

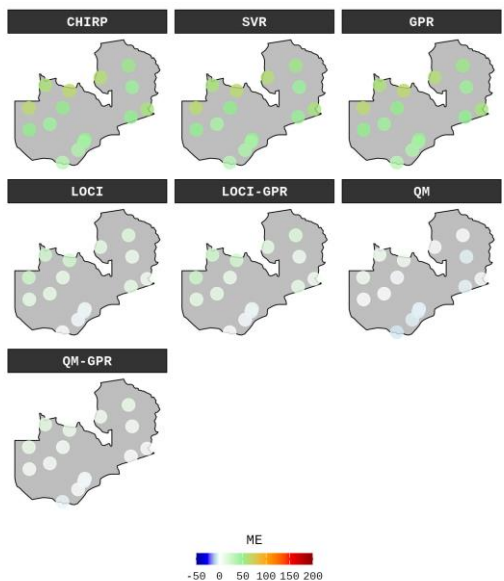

Figure S9: MEs on the annual number of rainy days across different stations in Zambia when the BC methods were applied on CHIRP

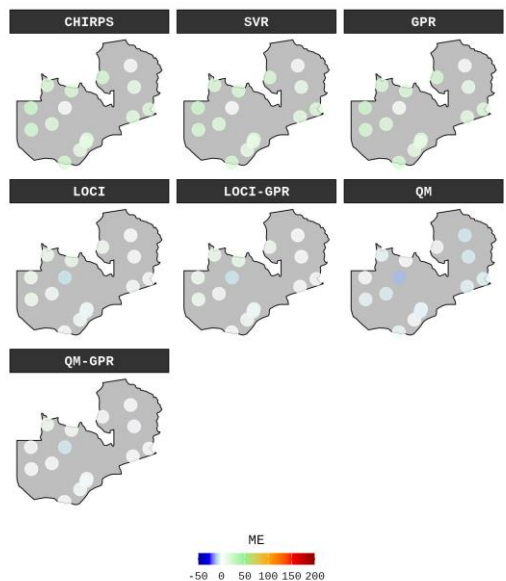

Figure S10: MEs on the annual number of rainy days across different stations in Zambia when the BC methods were applied on CHIRPS

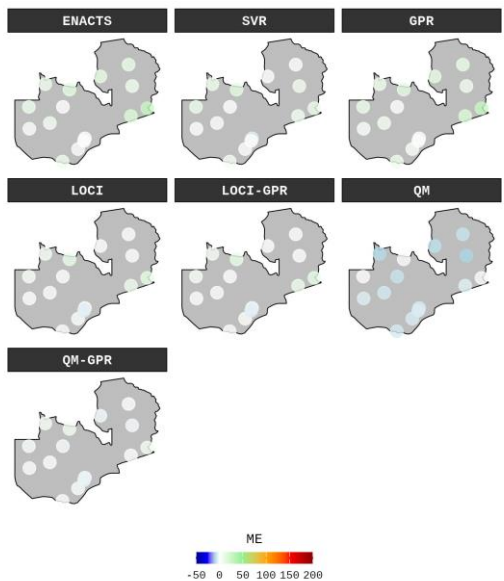

Figure S11: MEs on the annual number of rainy days across different stations in Zambia when the BC methods were applied on ENACTS

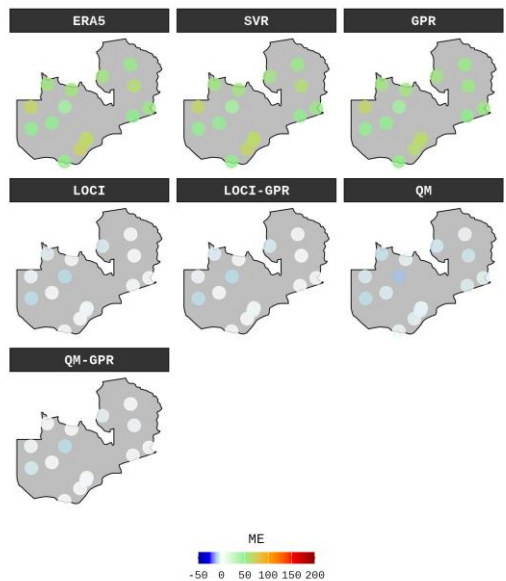

Figure S12: MEs on the annual number of rainy days across different stations in Zambia when the BC methods were applied on ERA5

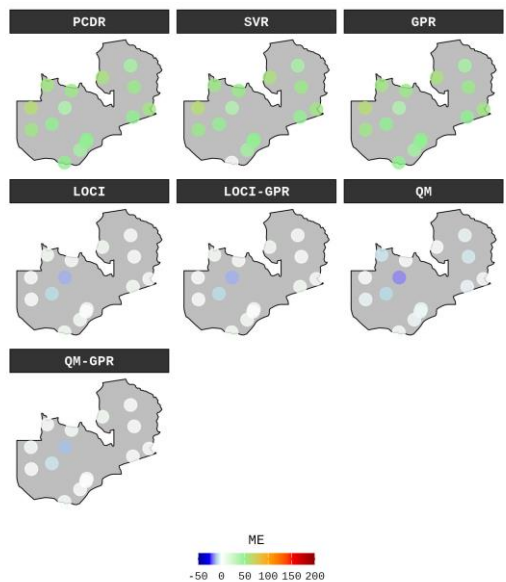

Figure 13: MEs on the annual number of rainy days across different stations in Zambia when the BC methods were applied on PCDR

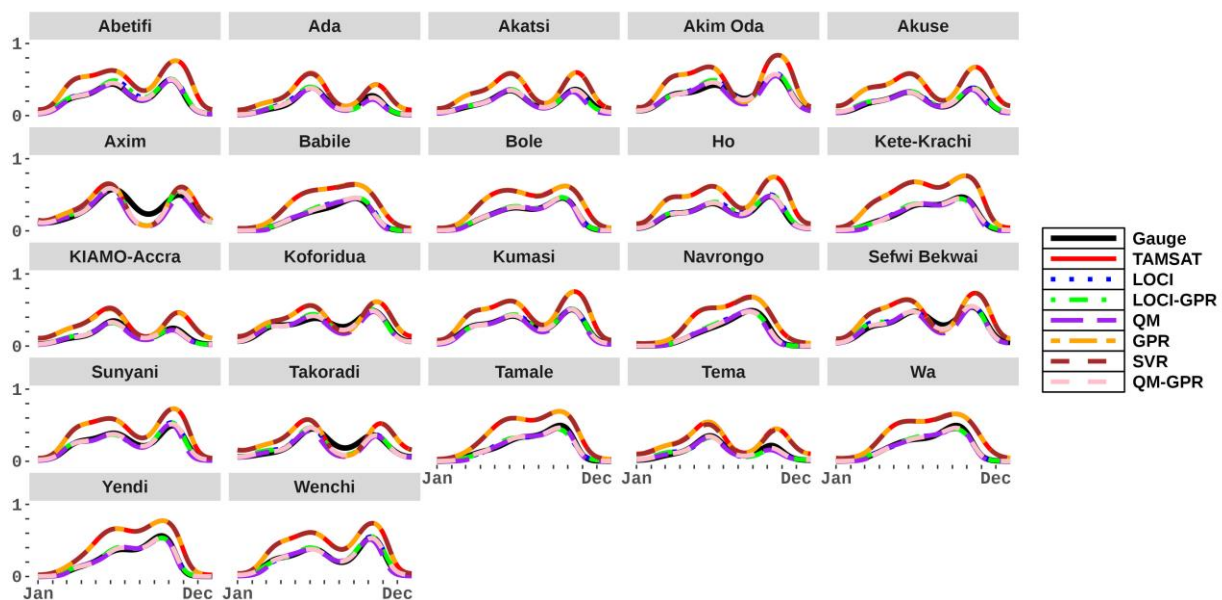

Figure S14: Performance of the BC methods on TAMSAT for capturing rainfall seasonality across the stations in Ghana. The y-axis represents the probability of rain, while the x-axis represents the day of year (January - December)



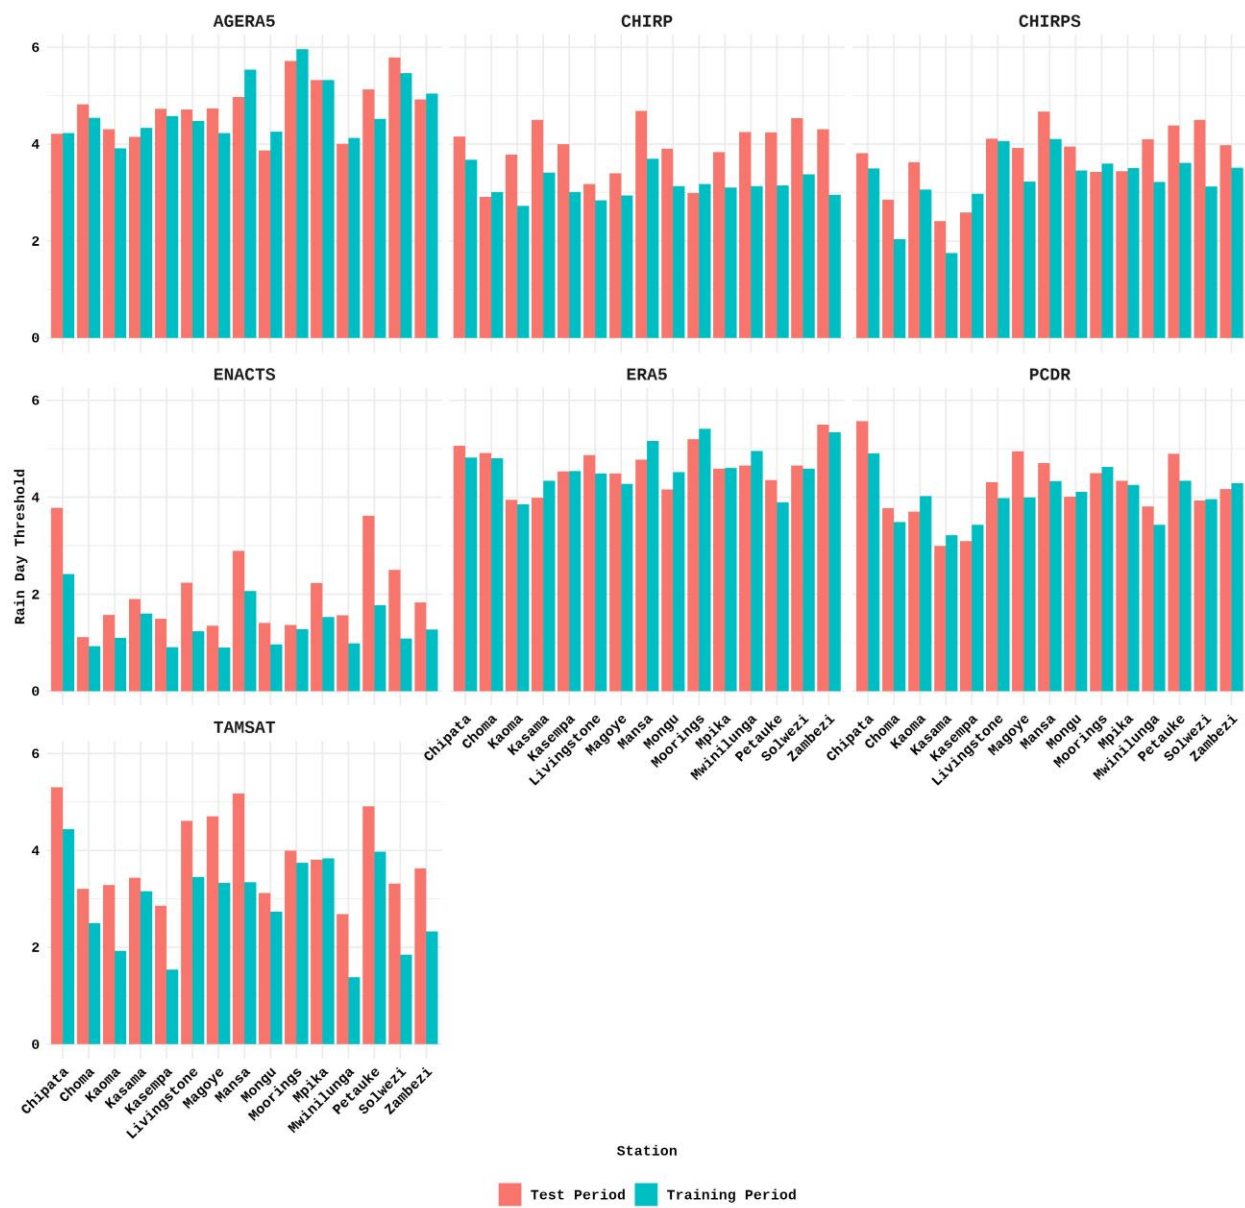

Figure S16: A grouped bar chart showing the fitted rain day thresholds of the SREs for the training period (1983 - 2000) applied on the test period vs the actual rain day threshold for the test period ( $\geq 2001$ ) across the stations and SREs in Zambia

Table S3: Performance metrics on annual total rainfall by SRE and BC methods in Zambia

| Product | Model | ME     | MAE   | RMSE  | Corr  | NSE    | RSD   |
|---------|-------|--------|-------|-------|-------|--------|-------|
| CHIRPS  | SRE   | -43.2  | 144.1 | 203.1 | 0.745 | 0.518  | 0.873 |
| CHIRPS  | GPR   | -228.9 | 241.9 | 300.8 | 0.746 | -0.058 | 0.702 |
| CHIRPS  | LOCI  | -4.9   | 164   | 225.7 | 0.695 | 0.404  | 0.974 |

|        |          |        |       |       |       |        |       |
|--------|----------|--------|-------|-------|-------|--------|-------|
| CHIRPS | LOCI-GPR | -291.3 | 301   | 356.6 | 0.711 | -0.487 | 0.721 |
| CHIRPS | QM       | 39.8   | 204   | 284.2 | 0.654 | 0.056  | 1.248 |
| CHIRPS | QM-GPR   | -302   | 310.7 | 364.6 | 0.716 | -0.554 | 0.713 |
| CHIRPS | SVR      | -668.3 | 668.3 | 703.3 | 0.698 | -4.783 | 0.477 |
| CHIRP  | SRE      | -40.6  | 195.9 | 254.7 | 0.64  | 0.242  | 1.025 |
| CHIRP  | GPR      | -115.5 | 194.6 | 253.8 | 0.675 | 0.247  | 0.906 |
| CHIRP  | LOCI     | 40.2   | 239.2 | 299.7 | 0.599 | -0.05  | 1.223 |
| CHIRP  | LOCI-GPR | -317.2 | 331.6 | 392.3 | 0.636 | -0.799 | 0.801 |
| CHIRP  | QM       | 5      | 253.3 | 313.5 | 0.586 | -0.149 | 1.287 |
| CHIRP  | QM-GPR   | -358.6 | 368.6 | 425.1 | 0.635 | -1.113 | 0.754 |
| CHIRP  | SVR      | -681.9 | 681.9 | 721.1 | 0.621 | -5.079 | 0.457 |
| ERA5   | SRE      | 49.1   | 169   | 217.3 | 0.691 | 0.448  | 0.73  |
| ERA5   | GPR      | -98.1  | 164.3 | 227.6 | 0.712 | 0.394  | 0.709 |
| ERA5   | LOCI     | -3     | 180.7 | 235.1 | 0.653 | 0.354  | 0.924 |
| ERA5   | LOCI-GPR | -332   | 335.5 | 393.9 | 0.692 | -0.814 | 0.629 |
| ERA5   | QM       | 119.9  | 257.3 | 320.6 | 0.614 | -0.202 | 1.256 |
| ERA5   | QM-GPR   | -307   | 341.3 | 400.2 | 0.565 | -0.873 | 0.863 |
| ERA5   | SVR      | -631.7 | 631.7 | 675.1 | 0.612 | -4.328 | 0.418 |
| TAMSAT | SRE      | -29.5  | 155.9 | 223   | 0.674 | 0.422  | 0.828 |
| TAMSAT | GPR      | -115.9 | 176.9 | 246.2 | 0.672 | 0.295  | 0.705 |
| TAMSAT | LOCI     | -29.4  | 163.8 | 237.6 | 0.62  | 0.344  | 0.799 |
| TAMSAT | LOCI-GPR | -204.7 | 230.9 | 307   | 0.636 | -0.096 | 0.752 |
| TAMSAT | QM       | 10.4   | 189.9 | 256.9 | 0.585 | 0.233  | 0.917 |
| TAMSAT | QM-GPR   | -220   | 240.6 | 314.4 | 0.647 | -0.149 | 0.721 |
| TAMSAT | SVR      | -550.8 | 550.8 | 598.8 | 0.599 | -3.168 | 0.553 |
| ENACTS | SRE      | -129.6 | 153.1 | 202.3 | 0.845 | 0.546  | 0.83  |

|        |          |        |       |       |       |        |       |
|--------|----------|--------|-------|-------|-------|--------|-------|
| ENACTS | GPR      | -40.7  | 116.7 | 166.9 | 0.831 | 0.691  | 0.87  |
| ENACTS | LOCI     | 13.1   | 112.8 | 158.3 | 0.84  | 0.722  | 0.867 |
| ENACTS | LOCI-GPR | -48.6  | 120.3 | 173.1 | 0.822 | 0.668  | 0.88  |
| ENACTS | QM       | -6.8   | 114.7 | 158.7 | 0.842 | 0.721  | 0.916 |
| ENACTS | QM-GPR   | -56.5  | 122.3 | 175.7 | 0.823 | 0.658  | 0.893 |
| ENACTS | SVR      | -162.4 | 183.6 | 234   | 0.815 | 0.393  | 0.839 |
| PCDR   | SRE      | -48.4  | 169.6 | 233.9 | 0.635 | 0.408  | 0.648 |
| PCDR   | GPR      | -89.4  | 163.4 | 227.6 | 0.708 | 0.439  | 0.759 |
| PCDR   | LOCI     | -61.3  | 188.6 | 257.7 | 0.598 | 0.282  | 0.877 |
| PCDR   | LOCI-GPR | -282.8 | 291.4 | 362.8 | 0.643 | -0.424 | 0.702 |
| PCDR   | QM       | -1.8   | 199.7 | 275.6 | 0.579 | 0.178  | 1.041 |
| PCDR   | QM-GPR   | -288.1 | 296.2 | 365.2 | 0.654 | -0.443 | 0.708 |
| PCDR   | SVR      | -605.6 | 605.6 | 648.9 | 0.638 | -3.555 | 0.484 |
| AGERA5 | SRE      | 72.6   | 195.1 | 245.6 | 0.618 | 0.295  | 0.775 |
| AGERA5 | GPR      | -108.9 | 170.9 | 235.7 | 0.7   | 0.351  | 0.712 |
| AGERA5 | LOCI     | -15.2  | 185.5 | 244.6 | 0.626 | 0.3    | 0.925 |
| AGERA5 | LOCI-GPR | -354.9 | 358.2 | 417.2 | 0.662 | -1.035 | 0.635 |
| AGERA5 | QM       | 101.7  | 252.2 | 321.5 | 0.584 | -0.208 | 1.239 |
| AGERA5 | QM-GPR   | -356.7 | 359.5 | 416.9 | 0.676 | -1.032 | 0.635 |
| AGERA5 | SVR      | -660.4 | 660.4 | 702.3 | 0.611 | -4.767 | 0.409 |

Table S4: Performance metrics on annual total rainfall by SRE and BC methods in Ghana

| Product | Model | ME     | MAE   | RMSE  | Corr  | NSE    | RSD   |
|---------|-------|--------|-------|-------|-------|--------|-------|
| CHIRPS  | SRE   | -47.4  | 158.7 | 205   | 0.773 | 0.541  | 0.952 |
| CHIRPS  | GPR   | -443.1 | 443.1 | 482.6 | 0.782 | -1.543 | 0.676 |
| CHIRPS  | LOCI  | -112.6 | 197.1 | 258.2 | 0.682 | 0.272  | 0.914 |

|         |          |        |       |       |       |        |       |
|---------|----------|--------|-------|-------|-------|--------|-------|
| CHIRPS  | LOCI-GPR | -559.8 | 559.8 | 592   | 0.796 | -2.827 | 0.6   |
| CHIRPS  | QM       | -63    | 227.6 | 292.9 | 0.606 | 0.064  | 1.116 |
| CHIRPS  | QM-GPR   | -557.7 | 557.7 | 589   | 0.804 | -2.788 | 0.606 |
| CHIRPS  | SVR      | -935.5 | 935.5 | 968.2 | 0.767 | -9.235 | 0.249 |
| CHIRP   | SRE      | -145.6 | 194.7 | 244.8 | 0.763 | 0.346  | 0.827 |
| CHIRP   | GPR      | -267.7 | 281.4 | 338.8 | 0.768 | -0.253 | 1.012 |
| CHIRP   | LOCI     | -168.9 | 292.8 | 634.2 | 0.394 | -3.215 | 2.192 |
| CHIRP   | LOCI-GPR | -633.8 | 633.8 | 661.7 | 0.784 | -3.588 | 0.762 |
| CHIRP   | QM       | -131.8 | 240.5 | 299.3 | 0.732 | 0.022  | 1.301 |
| CHIRP   | QM-GPR   | -622.3 | 622.3 | 650.4 | 0.782 | -3.618 | 0.747 |
| CHIRP   | SVR      | -903.4 | 903.4 | 936.1 | 0.688 | -8.566 | 0.328 |
| AGERAS5 | SRE      | -106.6 | 222.1 | 274.4 | 0.637 | 0.178  | 0.96  |
| AGERAS5 | GPR      | -200.3 | 226.1 | 276.2 | 0.795 | 0.167  | 0.961 |
| AGERAS5 | LOCI     | -50.5  | 241.3 | 312   | 0.666 | -0.063 | 1.357 |
| AGERAS5 | LOCI-GPR | -623.7 | 623.7 | 652.7 | 0.778 | -3.651 | 0.684 |
| AGERAS5 | QM       | 208.4  | 350.8 | 491.8 | 0.617 | -1.64  | 1.86  |
| AGERAS5 | QM-GPR   | -206.6 | 453.2 | 540.4 | 0.582 | -2.188 | 2.018 |
| AGERAS5 | SVR      | -873   | 873   | 907.8 | 0.662 | -7.997 | 0.323 |
| ERA5    | SRE      | -99.1  | 208.6 | 258.3 | 0.718 | 0.382  | 1.058 |
| ERA5    | GPR      | -152.8 | 194.4 | 241.6 | 0.814 | 0.459  | 0.983 |
| ERA5    | LOCI     | -40.5  | 252.8 | 325.9 | 0.663 | 0.016  | 1.421 |
| ERA5    | LOCI-GPR | -581.7 | 581.7 | 614.9 | 0.776 | -2.503 | 0.743 |
| ERA5    | QM       | 222.6  | 379.1 | 522.4 | 0.633 | -1.529 | 1.997 |
| ERA5    | QM-GPR   | -42.9  | 415.8 | 530.2 | 0.694 | -1.605 | 2.3   |
| ERA5    | SVR      | -840.5 | 840.5 | 880.2 | 0.644 | -6.179 | 0.331 |
| PCDR    | SRE      | -2.2   | 153.6 | 200.1 | 0.62  | 0.676  | 0.752 |

|        |          |        |       |       |       |        |       |
|--------|----------|--------|-------|-------|-------|--------|-------|
| PCDR   | GPR      | -188.5 | 209.8 | 250.2 | 0.709 | 0.493  | 0.607 |
| PCDR   | LOCI     | -140.6 | 202.8 | 256.1 | 0.534 | 0.468  | 0.697 |
| PCDR   | LOCI-GPR | -527.4 | 527.4 | 554.1 | 0.679 | -1.488 | 0.498 |
| PCDR   | QM       | -62.3  | 207.3 | 266   | 0.473 | 0.427  | 0.888 |
| PCDR   | QM-GPR   | -519.2 | 519.2 | 545.1 | 0.697 | -1.408 | 0.514 |
| PCDR   | SVR      | -863.4 | 863.4 | 884.5 | 0.618 | -5.341 | 0.269 |
| TAMSAT | SRE      | 16     | 159.2 | 204.6 | 0.759 | 0.564  | 0.91  |
| TAMSAT | GPR      | -109.2 | 167.6 | 214   | 0.804 | 0.523  | 0.899 |
| TAMSAT | LOCI     | 31.8   | 159.4 | 202.1 | 0.8   | 0.574  | 1.066 |
| TAMSAT | LOCI-GPR | -293.1 | 298.5 | 340.8 | 0.825 | -0.211 | 0.892 |
| TAMSAT | QM       | 108    | 227.4 | 296.3 | 0.682 | 0.084  | 1.224 |
| TAMSAT | QM-GPR   | -309.9 | 313.7 | 355.5 | 0.824 | -0.318 | 0.876 |
| TAMSAT | SVR      | -701.2 | 701.2 | 736.4 | 0.717 | -4.654 | 0.491 |
